# Supplementary material for: CARD: Controlled Agentic Reddit Discussions for Credit Card Simulation
Source: arXiv:2608.09790 source file (2026-08-11)
Supplement: Supplementary file 1 [file appendix.tex]

\section{Metric Calculation}
\label{sec:metrics_calculation}

\begin{table*}[t]
\centering
\scriptsize
\setlength{\tabcolsep}{0pt}
\renewcommand{\arraystretch}{1.18}

\caption{Detailed computation of thread-level evaluation metrics.
For a thread $T$, let $C_T=\{c_1,\ldots,c_m\}$ denote its comments,
$P_T=\{(i,j):1\le i<j\le m\}$ its unordered comment pairs, and
$R_T$ its parent--reply pairs.}
\label{tab:metric_computation_details}

\begin{tabularx}{\textwidth}{
  @{}
  L{0.155\textwidth}
  @{\hspace{8pt}}
  L{0.285\textwidth}
  @{\hspace{10pt}}
  Y
  @{}
}
\toprule
\textbf{Metric}
& \textbf{Thread-level formula}
& \textbf{Implementation details} \\
\midrule

Self-BLEU-4
&
$\displaystyle
\begin{aligned}
\phi_{\mathrm{SB}}(T)
&=
\frac{1}{|P_T|}
\sum_{(i,j)\in P_T}s_{ij},
\\[-2pt]
s_{ij}
&=
\frac{
\mathrm{BLEU}_4(c_i,c_j)
+
\mathrm{BLEU}_4(c_j,c_i)
}{2}
\end{aligned}$
&
Each comment is tokenized with a regex tokenizer and lowercased.
For every unordered comment pair, CARD computes BLEU in both
directions and averages the two scores. BLEU uses modified
$n$-gram precision up to order 4, add-one smoothing, and the
standard brevity penalty. Threads with fewer than two usable
comments receive score 0. \\
\addlinespace[2pt]

Self-BERTScore
&
$\displaystyle
\frac{1}{|P_T|}
\sum_{(i,j)\in P_T}
\mathrm{BERTScoreF1}(c_i,c_j)$
&
For each unordered comment pair, CARD computes BERTScore precision,
recall, and F1. The reported metric is the mean pairwise F1 within
the thread. The default model is
\path{microsoft/deberta-xlarge-mnli}, with
\path{roberta-large} as fallback. \\
\addlinespace[2pt]

Mean semantic cosine
&
$\displaystyle
\frac{1}{|P_T|}
\sum_{(i,j)\in P_T}
\cos(e_i,e_j)$
&
Each comment is encoded with
\path{sentence-transformers/all-mpnet-base-v2}.
Embeddings are normalized, and the thread score is the mean cosine
similarity over all unordered comment pairs. If
\texttt{sentence-transformers} is unavailable, CARD uses the same
transformer with attention-mask mean pooling. \\
\addlinespace[2pt]

Hard disagreement rate
&
$\displaystyle
\frac{1}{|R_T|}
\sum_{(p,r)\in R_T}
\mathbf{1}
\{\hat y_{p,r}=\mathrm{disagree}\}$
&
For each reply, CARD forms a parent--reply pair. The parent is the
root post for a top-level comment and the parent comment for a nested
reply. A local Stance\_Rel RoBERTa classifier predicts
\texttt{disagree}, \texttt{neutral}, or \texttt{agree}. The metric is
the fraction predicted as \texttt{disagree}. \\
\addlinespace[2pt]

Politeness rate
&
$\displaystyle
\frac{1}{m}
\sum_{i=1}^{m}
\mathbf{1}\{\hat y_i=\mathrm{polite}\}$
&
Each comment is classified independently using
\path{Intel/polite-guard}. The classifier predicts
\texttt{polite}, \texttt{somewhat\_polite}, \texttt{neutral}, or
\texttt{impolite}. The metric is the fraction whose predicted label
is exactly \texttt{polite}. \\
\addlinespace[2pt]

Impoliteness rate
&
$\displaystyle
\frac{1}{m}
\sum_{i=1}^{m}
\mathbf{1}\{\hat y_i=\mathrm{impolite}\}$
&
Using the same per-comment predictions, the metric is the fraction
of comments predicted as \texttt{impolite}. \\
\addlinespace[2pt]

Neutral rate
&
$\displaystyle
\frac{1}{m}
\sum_{i=1}^{m}
\mathbf{1}\{\hat y_i=\mathrm{neutral}\}$
&
Using the same per-comment predictions, the metric is the fraction
of comments predicted as \texttt{neutral}. The
\texttt{somewhat\_polite} class is not included as a reported
comparison metric. \\
\addlinespace[2pt]

Length CV
&
$\displaystyle
\frac{
\sigma(\ell_1,\ldots,\ell_m)
}{
\mu(\ell_1,\ldots,\ell_m)
}$
&
For each comment, $\ell_i$ is its whitespace-token count. CARD
divides the population standard deviation of comment lengths by
their mean. If the mean is zero, the score is set to 0. \\
\addlinespace[2pt]

Average reply depth
&
$\displaystyle
\frac{1}{m}
\sum_{i=1}^{m}d_i$
&
CARD reconstructs the reply tree from parent ids. Top-level comments
have depth 1, and each child has depth one greater than its parent.
The metric is the mean depth across comments. \\
\addlinespace[2pt]

Structural virality
&
$\displaystyle
\frac{1}{|P_T|}
\sum_{(i,j)\in P_T}
\operatorname{dist}_{T}(c_i,c_j)$
&
CARD treats the comment tree as an undirected graph over comments.
It computes the shortest-path distance between each unordered
comment pair and reports the mean. Threads with fewer than two
comments receive score 0. \\
\addlinespace[2pt]

Mean story probability
&
$\displaystyle
\frac{1}{m}
\sum_{i=1}^{m}
p_{\mathrm{story}}(c_i)$
&
Each comment is scored with \path{mariaantoniak/storyseeker}.
The metric is the mean \texttt{story} probability across comments,
rather than the fraction above a fixed threshold. \\
\addlinespace[2pt]

Emotion entropy
&
$\displaystyle
-\sum_{e\in\mathcal E}
q_e\log q_e$
&
Each comment is scored with
\path{SamLowe/roberta-base-go_emotions}. CARD uses the
highest-probability label as the dominant emotion and computes the
empirical distribution $q_e$ of dominant emotions within the thread.
The reported value is Shannon entropy using natural logarithms. \\

\bottomrule
\end{tabularx}
\end{table*}

\newpage
\begin{table*}[t]
\centering
\scriptsize
\setlength{\tabcolsep}{2.2pt}
\resizebox{\textwidth}{!}{
\begin{tabular}{llcccccccccccccccccccccccc}
\toprule
\multirow{2}{*}{Method} & \multirow{2}{*}{Model}
& \multicolumn{2}{c}{Self-BLEU}
& \multicolumn{2}{c}{Self-BERT}
& \multicolumn{2}{c}{Sem. Cos.}
& \multicolumn{2}{c}{Hard Dis.}
& \multicolumn{2}{c}{Polite}
& \multicolumn{2}{c}{Impolite}
& \multicolumn{2}{c}{Neutral}
& \multicolumn{2}{c}{Len. CV}
& \multicolumn{2}{c}{Depth}
& \multicolumn{2}{c}{Virality}
& \multicolumn{2}{c}{Story}
& \multicolumn{2}{c}{Emotion} \\
\cmidrule(lr){3-4}
\cmidrule(lr){5-6}
\cmidrule(lr){7-8}
\cmidrule(lr){9-10}
\cmidrule(lr){11-12}
\cmidrule(lr){13-14}
\cmidrule(lr){15-16}
\cmidrule(lr){17-18}
\cmidrule(lr){19-20}
\cmidrule(lr){21-22}
\cmidrule(lr){23-24}
\cmidrule(lr){25-26}
& & Cliff & W
& Cliff & W
& Cliff & W
& Cliff & W
& Cliff & W
& Cliff & W
& Cliff & W
& Cliff & W
& Cliff & W
& Cliff & W
& Cliff & W
& Cliff & W \\
\midrule

\multirow{4}{*}{OASIS}
& gemini-2.5-flash
& 0.421 & 0.0155
& 0.863 & 0.0863
& 0.827 & 0.2967
& 0.444 & 0.1634
& 0.744 & 0.4129
& -0.347 & 0.1316
& -0.736 & 0.1779
& -0.511 & 0.2837
& -0.836 & 1.0080
& -0.836 & 1.7780
& -0.866 & 0.1440
& 0.259 & 0.2461 \\

& deepseek-v4-flash
& 0.497 & 0.0236
& 0.685 & 0.1056
& 0.718 & 0.3655
& 0.269 & 0.1455
& 0.749 & 0.4672
& -0.507 & 0.2061
& -0.740 & 0.1787
& -0.828 & 0.5139
& -0.841 & 1.0420
& -0.836 & 1.7780
& -0.548 & 0.1071
& -0.141 & 0.1474 \\

& gpt-4o-mini
& 0.672 & 0.0790
& 0.680 & 0.2049
& 0.679 & 0.4174
& 0.196 & 0.0618
& 0.793 & 0.5515
& -0.787 & 0.3498
& -0.719 & 0.1741
& -0.895 & 0.6396
& -0.847 & 1.0760
& -0.836 & 1.7780
& -0.860 & 0.1445
& -0.134 & 0.1404 \\

& gpt-5.4-mini
& 0.553 & 0.0740
& 0.560 & 0.1979
& 0.560 & 0.3589
& -0.131 & 0.0564
& 0.296 & 0.1916
& -0.351 & 0.1453
& -0.714 & 0.1733
& -0.890 & 0.6268
& -0.859 & 1.1520
& -0.836 & 1.7780
& -0.967 & 0.1529
& -0.318 & 0.3264 \\

\midrule

\multirow{4}{*}{SynthPAI}
& gemini-2.5-flash
& 0.938 & 0.0621
& 0.766 & 0.0651
& -0.090 & 0.0307
& 0.480 & 0.1231
& -0.761 & 0.2825
& 0.824 & 0.3969
& -0.129 & 0.0414
& -0.738 & 0.3736
& 0.111 & 0.2598
& 0.087 & 0.3154
& -0.516 & 0.1178
& -0.303 & 0.2624 \\

& deepseek-v4-flash
& 0.898 & 0.0599
& 0.742 & 0.0644
& 0.144 & 0.0318
& 0.337 & 0.0954
& -0.736 & 0.2742
& 0.796 & 0.4128
& -0.293 & 0.0738
& -0.046 & 0.0739
& -0.011 & 0.2250
& 0.037 & 0.3175
& \best{0.075} & 0.0336
& -0.359 & 0.3304 \\

& gpt-4o-mini
& 0.737 & 0.0210
& 0.923 & 0.1028
& 0.254 & 0.0484
& 0.235 & 0.0703
& -0.352 & 0.1390
& 0.749 & 0.3465
& -0.638 & 0.1508
& -0.599 & 0.3062
& \best{0.009} & 0.2470
& \best{-0.010} & 0.3267
& -0.603 & 0.1268
& 0.023 & 0.0987 \\

& gpt-5.4-mini
& 0.959 & 0.0599
& 0.882 & 0.0827
& \best{0.012} & 0.0216
& 0.252 & 0.0360
& -0.738 & 0.2823
& 0.794 & 0.3775
& -0.206 & 0.0575
& 0.235 & 0.2111
& 0.418 & 0.5896
& 0.443 & 0.8802
& -0.319 & 0.0923
& -0.318 & 0.3199 \\

\midrule

\multirow{4}{*}{CARD}
& gemini-2.5-flash
& 0.094 & 0.0048
& 0.238 & 0.0317
& \best{0.007} & 0.0245
& 0.075 & 0.0207
& \best{0.044} & \best{0.0222}
& -0.329 & 0.1354
& 0.060 & 0.0270
& -0.057 & 0.0624
& 0.112 & 0.1655
& 0.128 & 0.2731
& \best{0.002} & \best{0.0135}
& 0.124 & 0.1133 \\

& deepseek-v4-flash
& \best{0.058} & 0.0031
& \best{-0.002} & 0.0115
& -0.074 & 0.0178
& -0.046 & 0.0228
& -0.077 & 0.0335
& 0.046 & \best{0.0211}
& \best{-0.016} & \best{0.0199}
& \best{0.041} & 0.0580
& -0.037 & \best{0.0720}
& -0.050 & \best{0.1163}
& 0.157 & 0.0332
& -0.018 & 0.0523 \\

& gpt-4o-mini
& 0.155 & 0.0038
& 0.676 & 0.0535
& 0.164 & 0.0411
& 0.142 & 0.0566
& \best{0.063} & \best{0.0290}
& -0.116 & 0.0518
& -0.198 & 0.0520
& -0.147 & 0.1060
& -0.117 & 0.1907
& -0.127 & 0.2602
& 0.096 & 0.0310
& 0.233 & 0.2412 \\

& gpt-5.4-mini
& 0.069 & \best{0.0018}
& 0.068 & \best{0.0102}
& -0.058 & \best{0.0160}
& \best{0.043} & \best{0.0185}
& -0.198 & 0.0892
& \best{0.035} & 0.0217
& -0.088 & 0.0238
& -0.058 & \best{0.0576}
& -0.075 & 0.1168
& -0.100 & 0.2286
& -0.076 & \best{0.0243}
& \best{0.009} & \best{0.0413} \\

\bottomrule
\end{tabular}
}
\caption{
Effect-size and distribution-distance comparison across methods and models.
Cliff's $\delta$ reports the direction and magnitude of distributional
shift, while Wasserstein distance reports absolute distributional distance.
Values closer to zero indicate better agreement with real discussions.
Green-highlighted cells indicate the smallest absolute Cliff's $\delta$
or the smallest Wasserstein distance in each column.
}
\label{tab:effect_distance_results}
\end{table*}
